# Supplementary material for: ROPocop - Dynamic Mitigation of Code-Reuse Attacks
Source: arXiv:1504.02288 source file (2015-04-09)
Supplement: Supplementary file 1 [file 10-Appendix.tex]

\begin{lstlisting}[language=C++, caption=Vulnerable C program, label=vulnProg,
float] 
#include "stdafx.h"
#include <stdio.h>

void foo_vuln(char* str)
{
	char buffer[12];
	strcpy(buffer, str); //unbounded strcpy!
	printf("%s\n", buffer);
}

int main(int argc, char* argv[])
{
	char locBuf[64];
	foo_vuln(argv[1]);
	return 0;
}
\end{lstlisting}

\begin{lstlisting}[language=Perl, caption=Exploit for our
vulnerable program in Perl, label=vulnProgExploit, numbers=none, float]
my $nops = "\x90" x 12;
my $ebp = "\x41" x 4;
my $ret = "\x8C\xFE\x18\x00";
my $exp = $nops.$ebp.$ret;
\end{lstlisting}

\begin{table*}
\centering

\rowcolors{3}{black!10}{}
    \begin{tabular}{c | p{9cm} | p{1.60cm} p{1.60cm} p{1.25cm} | p{1.25cm}}
    \rowcolor{black!20}
    \textbf{ID} & \textbf{Exploit name} & \textbf{Indirect Branches, threshold:
    35} &
    \textbf{Average BB-Length, threshold: 2.25} & \textbf{Detected by AntiCRA} 
    & \textbf{Detected by DEP+} \\
    E01 & ASX to MP3 Converter v3.1.2.1 SEH Exploit (Multiple OS, DEP and ASLR
    Bypass) & \textbf{\textgreater 50} & \textgreater 2.25 & Yes & Yes \\
    E02 & BlazeDVD 5.1 Stack Buffer Overflow With ASLR/DEP Bypass &
    20 & \textbf{1.9} & Yes & Yes \\
    E03 & BlazeDVD 6.1 PLF Exploit DEP/ASLR Bypass & 16 & \textbf{2} & Yes & Yes 
    \\
    E04 & DVD X Player 5.5.0 Pro / Standard version Universal Exploit, DEP+ASLR
    Bypass & 17 & \textbf{2} & Yes & Yes \\
    E05 & DVD X Player 5.5 Pro (SEH DEP + ASLR Bypass) Exploit & 13 & (2.2)* &
    No & Yes \\
    E06 & ProSSHD 1.2 remote post-auth exploit (w/ASLR and DEP bypass) & \textbf{43} &
    \textbf{2} & Yes & Yes \\
    E07 & RM Downloader 3.1.3 Local SEH Exploit (Win7 ASLR and DEP Bypass) &
    \textbf{49} & \textgreater 2.25 & Yes & Yes \\
    E08 & The KMPlayer 3.0.0.1440 .mp3 Buffer Overflow Exploit (Win7 + ASLR bypass
    mod) & \textbf{46} & \textgreater 2.25 & Yes & Yes \\
    E09 & UFO: Alien Invasion v2.2.1 BoF Exploit (Win7 ASLR and DEP Bypass) &
    \textbf{\textgreater 50} & \textgreater 2.25 & Yes & Yes \\
    E10 & Winamp v5.572 Local BoF Exploit (Win7 ASLR and DEP Bypass) &
    \textbf{\textgreater 50} & \textbf{2} & Yes & Yes \\
    E11 & Adobe Reader 11.0.01 ``Number of the Beast'' (ASLR, DEP, Sandbox
    bypass, pure RoP)** & \textbf{\textgreater 50} & - & Yes & No \\
    E12 & QQ PLAYER PICT PnSize Buffer Overflow WIN7 DEP ASLR BYPASS & 11 & (2)*
    & No & Yes \\
    \end{tabular}
* not computed by AntiCRA due to low number of indirect branches ($<$15)

** data is based on the analysis by Li and Szor~\cite{reader_666}
\vspace{0.5em}    
\caption{Analysis of Exploits}
\label{tab:eval_exploits}
\end{table*}

Figures~\ref{fig:indbra} and \ref{fig:bbllength} give additional raw data for
the data points summarized by Figure~\ref{fig:scatterplot}.

\pgfplotstableread{ % Read the data into a table macro
Label   IndBranch	BBL
E1		50			2.5
E2		20			1.9
E3		16			2
E4		17			2
E5		13			0
E6		43			2
E7		49			2.5
E8		46			2.5
E9		50			2.5
E10		50			2
E11		50			0
E12		11			2
400		4			0
401		3			0
403		6			0
429		3			0
433		3			0 
444		4			0
445		5			0
447		7			0
450		8			0
453		6			0 
456		3			0
458		3			0
464		31			4
470		4			0
471		15			3.91
473		3			0
482		9			0
483		17			4
Filezilla	14		2.5
VLC		14			2.6
Reader	29			2.33
}\datatable

%464: BBL :  %9.91
%483: BBL :  %4.3

\begin{figure*}
\begin{tikzpicture}
  \begin{axis}[
   	axis x line=bottom,
    axis y line=left,
    ybar,
    height=6cm,
    width=\linewidth,
    ylabel=No. of indirect branches in a row,
    xtick=data,
    xticklabels from table={\datatable}{Label},
    xlabel=Evaluated exploits and applications,
    every node near coord/.append style={font=\footnotesize},
    nodes near coords, 
	nodes near coords align={vertical},
    x tick label style={rotate=45,anchor=east},
    enlarge x limits=0.042,
    ]
    \addplot [fill=black!20] table [y=IndBranch, x expr=\coordindex]
{\datatable};
\draw[red] [thick] (-15,320) -- (320,320);
\draw[red] [thick] (115,-20) -- (115,520);
\node at (30,450) {Exploits};
\node at (210,450) {Benchmarks \& Applications};
\end{axis}
\end{tikzpicture}
\caption{Highest encountered number of consecutive indirect branches}
\label{fig:indbra}
\end{figure*}

\begin{figure*}
\begin{tikzpicture}
  \begin{axis}[
 	axis x line=bottom,
    axis y line=left,
    ybar, 
    height=6cm,
    width=\linewidth,
    ylabel=Lowest average of BBLs,
    xtick=data,
    every node near coord/.append style={font=\footnotesize},
    xticklabels from table={\datatable}{Label},
    xlabel=Evaluated exploits and applications,
    nodes near coords, 
    enlarge x limits=0.042,
	%nodes near coords align={vertical},
    x tick label style={rotate=45,anchor=east},
    ]
    \addplot [fill=black!20] table [y=BBL, x expr=\coordindex]
{\datatable};
\node at (50,370) {Exploits};
\node at (175,370) {Benchmarks \& Applications};
\draw[red] [thick] (-15,225) -- (320,225);
\draw[red] [thick] (115,-20) -- (115,520);
\end{axis}
\node [fill=white] at (2.59,0.27) {\footnotesize n/a};
\node [rectangle, minimum width=5.8cm, fill=white] at (9.20,0.27) {\footnotesize n/a};
\node [fill=white] at (12.78,0.27) {\footnotesize n/a};
\node [rectangle, minimum width=1cm, fill=white] at (14.00,0.27)
{\footnotesize n/a};
\end{tikzpicture}
\caption{Lowest average of basic block lengths after at least 15 consecutive
indirect branches}
\label{fig:bbllength}
\end{figure*}
